# Supplementary material for: STMARL: A Spatio-Temporal Multi-Agent Reinforcement Learning Approach for Cooperative Traffic Light Control
Source: arXiv:1908.10577 source file (2020-11-29)
Supplement: Supplementary file 1 [file sec_appendix.tex]

\subsection{Traffic Light Phase Configuration}
\begin{figure}[ht]
    \centering
    \includegraphics[height=0.6\vsize, width=1.0\hsize]{firgure/phase_config.pdf}
    \caption{Detailed phase configuration for the traffic lights used in the real-world dataset $D_{Hefei}$.}\label{fig:phase_detail_config}
\end{figure}
We provide all phases configuration used by the four traffic lights for the real-world dataset $D_{Hefei}$ in Figure~\ref{fig:phase_detail_config}. Each traffic light's phase id list is shown in Table~\ref{table:phase_config} in the main text.

\subsection{Road Network Setting}
For the synthetic data, each intersection has four directions and each road segment has 3 lanes (300 meters long and 3.2 meters width). The road network in the real data is imported from OpenStreetMap~\footnote{https://www.openstreetmap.org}.
